# Supplementary material for: Certificate Enhanced Data-Flow Analysis
Source: arXiv:1808.01246 source file (2018-08-03)
Supplement: Supplementary file 1 [file appendix.tex]

\centerline{\bf Appendix}
\bigskip

 To ease the usage of DSlicer we provide a virtual machine image including a tutorial (Demo) illustrating its usage. Please find the virtual machine under\\

 https://drive.google.com/open?id=0B42EyIYV28cpbmtHWXFSdElFVE0

\iffalse
%%%%%%%%%%%%%%%%%%%%%%%%%%%%%%%%%%%%%%%%%%%%%%%%%%%%%%%%%%%%%%%%%%%%%%%%%%%%%%%
\bigskip This is a brief demonstration of the usage and capabilities of DSlicer.

\bigskip
\noindent let us start by displaying the available option for DSlicer. This is done via 

\bigskip
\noindent
\begin{myvtim2} 
{\small
\hspace{-.4cm}python2.7  DroidGen.py -f examples/apps/Recorder.apk -m -r recorder.spec
}
\end{myvtim2}
%%%%%%%%%%%%%%%%%%%%%%%%%%%%%%%%%%%%%%%%%%%%%%%%%%%%%%%%%%%%%%%%%%%%%%%%%%%%%%%
\fi
